# Supplementary material for: Spatial heterogeneities in structural temperature cause Kovacs expansion gap paradox in aging of glasses
Source: arXiv:1909.03685 ancillary file (2019-09-09)
Supplement: Supplementary file 1 [file Kovacs_Gap_Supplemental.pdf]

# Supplemental: Spatial heterogeneities in structural temperature cause Kovacs' expansion gap paradox in aging of glasses

Matteo Lulli,[1] Chun-Shing Lee,[1] Hai-Yao Deng,[2] Cho-Tung Yip,[3] and Chi-Hang Lam[1]

[1]*Department of Applied Physics, Hong Kong Polytechnic University, Hong Kong, China*
[2]*School of Physics, University of Exeter, Exeter EX4 4QL, United Kingdom*
[3]*School of Science, Harbin Institute of Technology, Shenzhen Graduate School, Shenzhen, Guangdong 518055, China*

(Dated: September 9, 2019)

## I. THERMAL PROPERTIES OF DPLM

We report here some further details about the DPLM. In the main text, we discuss about the final equilibrium value of the system energy $E_\infty$ and the specific heat as a function of the temperature. Let us now derive in detail these two quantities. In order to obtain the equilibrium energy $E_\infty$ as a function of the temperature $T$ one has to compute the average of the system energy (see Eq.(1) in the main text)

$$E_\infty(T) = \sum_{\langle ij\rangle'} \langle V_{ijs_is_j}\rangle_T = N_b \int_{V_0}^{V_1} \mathrm{d}V\, V\, p_{eq}(V,T), \quad (1)$$

where $[V_0, V_1]$ is the range of variation of the couplings, $N_b$ is the average number of bonds and $p_{eq}$ is the equilibrium distribution of the interaction energies given in Eq.(2) of the main text. A good estimate of $N_b$, at a low void density, can be obtained in the approximation of isolated voids, i.e. a void does not have another void as a nearest neighbor, yielding in two dimensions $N_b = 2L^2 - 4N_v \simeq 2N(1-\phi_v)$, where $2L^2$ is the number of interactions for the fully occupied lattice while each isolated void decreases this number by the 4 missing couplings with its nearest neighboring particles. Hence, the problem reduces to computing the average interaction energy as a function of the temperature, i.e. $\langle V\rangle_T$. In this paper we choose $g(V)$ as a uniform distribution, i.e. $g(V) = 1/\Delta V$ where $\Delta V = V_1 - V_0$ is the range of variation of the interactions. Hence, choosing the boundary values as $V_1 = -V_0 = 1/2$ and keeping on using natural units as in the main text, we write

$$E_\infty(T) = 2N(1-\phi_v)\left[T - \frac{1}{2}\coth\left(\frac{1}{2T}\right)\right]. \quad (2)$$

It is easy to check that $E_\infty(T) \leq 0$ where the equality holds in the limit $T \to \infty$. By taking the derivative with respect to the temperature, we write the heat capacity as

$$C_V(T) = 2N(1-\phi_v)\left\{1 - \frac{1}{4T^2}\left[\coth^2\left(\frac{1}{2T}\right) - 1\right]\right\}, \quad (3)$$

which is a decreasing function of $T$.

## II. OVERLAP AND VOIDS DYNAMICS

In the main text, we report the evolution of different quantities, in Figures 2 and 3, as a function of the average overlap rather than as a function of time. This choice is motivated by the fact that the differences in the dynamics between down- and up-jump are most clearly visible when measuring the evolution in terms of the fraction of particles that at a given time $t$ still retain the position $\vec{x}_0$ at the moment when the temperature jump is performed, i.e. the average overlap $q$ as discussed in the main text. Hence, we report in Fig. 1 the evolution of the average overlap as a function of time, where the much slower up-jump relaxation is clearly visible.

Finally, we report the positions of the voids for three of the configurations shown in Fig.2 of the main text. We notice that for the down-jump dynamics all the voids belong to the mobile region already at an early stage, while for the up-jump some voids stay *trapped* in the immobile regions. The voids and fields dynamics can be examined also from the supplementary videos *supvideo_up.mp4* and *supvideo_down.mp4*.

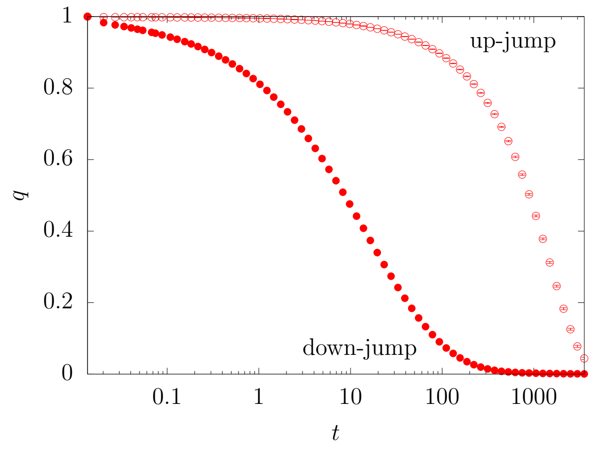


FIG. 1. Average overlap evolution, $q(t)$, for up-jump with $T_i = 0.1$ and down-jump with $T_i = 0.3125$, with a common final temperature $T_f = 0.25$. These values are the same as those used in Fig.2 of the main text.

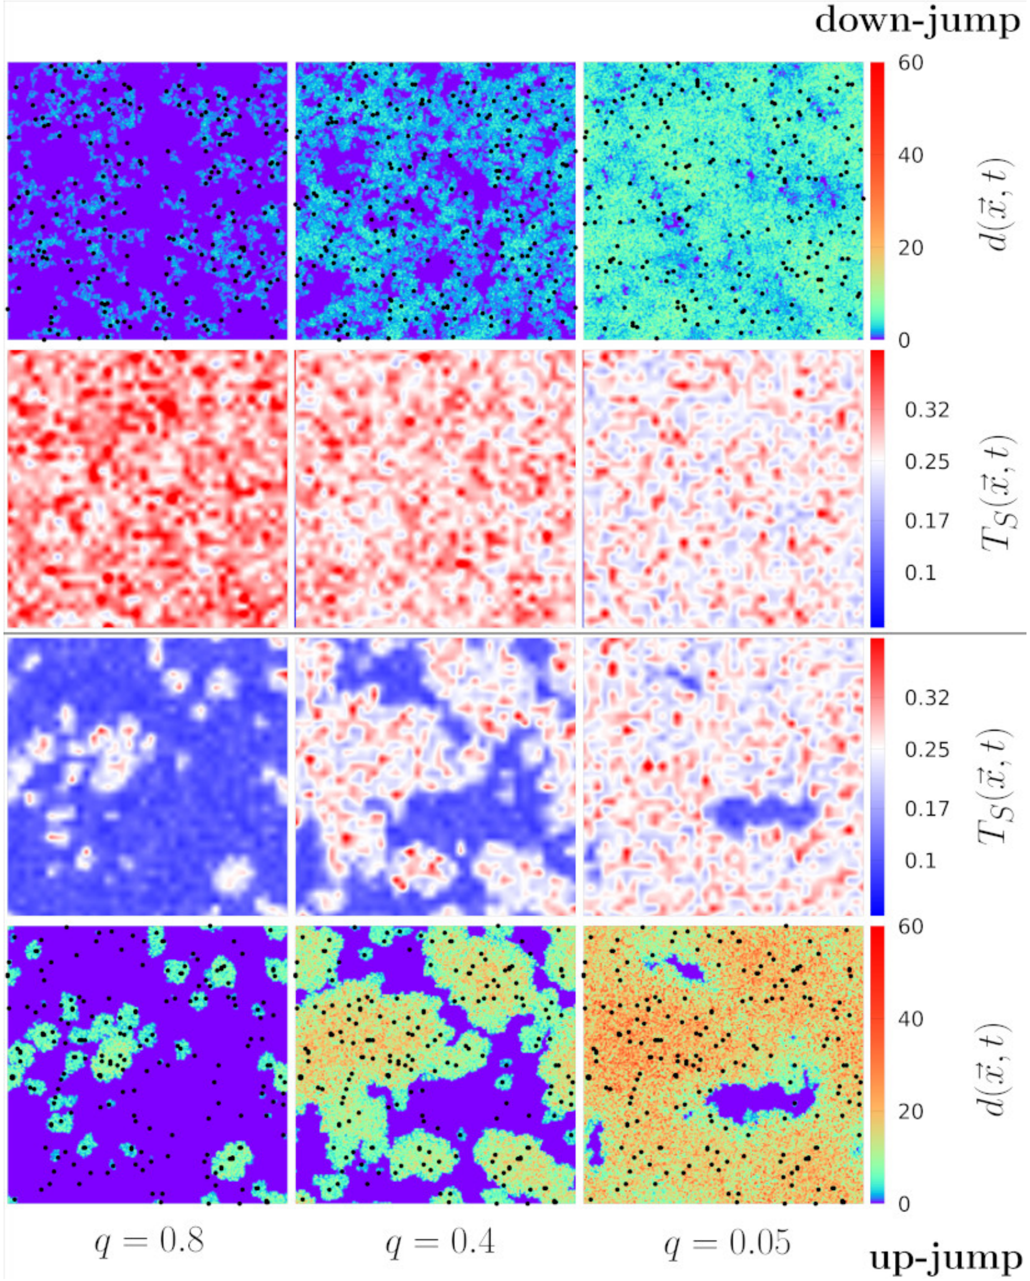


FIG. 2. Three of the four snapshots reported in Fig.1 of the main text with the voids positions reported by black dots. The initial temperatures are $T_i = 0.3125$ and $T_i = 0.1$ for the down- and up-jump respectively, with the final temperature $T_f = 0.25$.
